# Supplementary material for: Pika: Empowering Non-Programmers to Author Executable Governance Policies in Online Communities
Source: arXiv:2310.04329 source file (2024-02-27)
Supplement: Supplementary file 1 [file appendix.tex]

An important part of the declarative language is for policy components (\term{base action}, \term{filter}, \term{base procedure}, \term{decorator}, and \term{execution}). These policy components are designed to follow a consistent pattern. They are represented using JSON fields and are associated with a corresponding code snippet. These JSON fields allow users to configure a policy component, which subsequently is mapped to its associating code snippet in PolicyKit. To be precise, every policy component is defined by a set of JSON fields which include: an identifier (typically \code{name}), descriptive elements (such as \code{label} or \code{description}), \term{settings}, and \term{variables}. The descriptive elements introduce each policy component to end-users in natural language, while the \term{settings} provide guidance on its configuration (\dgone{}). 

\term{Settings} for policy components encompass the following JSON fields: \code{name} serves as the identifier, \code{label} provides descriptive information, and \code{type} details its data type (such as \code{string}, \code{number}, or \code{float}). % 

\term{Variables} of policy components have similar JSON fields. 
Settings also have a \code{required} attribute that indicates whether user input is necessary or not, and a \code{default} attribute that will be used when there is no user input.

Figure \ref{custom actions} (left) presents an example of \term{custom actions} in the form of declarative language. It specifies the \term{base action} this \term{custom action} builds upon (i.e., \code{SlackRenameChannel}) and enumerates \term{filters} designated for each field of this \term{base action}. Similar to other policy components, each \term{filter} has the following JSON fields:  \code{name}, \code{description}, \term{settings}, and \term{variables}. 

\begin{figure}[!h]
    \centering
    \includegraphics[width=\columnwidth]{figures/custom_action.pdf}
    % \includesvg[inkscapelatex=false,width=\columnwidth]{figures/custom_action.svg}
    % \includepdf[width=\columnwidth]{figures/custom_action.pdf}
    \caption{ (left) \textbf{An Example of Custom Actions} Here the \term{custom action} specifies the \term{base action} and \term{filters} used for each action field. Put them together, it governs actions when a user of the role \code{Base User} renames the Slack channel \code{\#general}. (middle) \textbf{An Example of Base Actions} It represents the generic action when a user renames a Slack channel. Its \term{variables} such as \code{initiator} and \code{channel} offer further information about it and could be referenced across policy components. (right) \textbf{An Example of Filters} This \term{filter} is used to determine whether a user has the specified role. }
    \hfill
    \label{custom actions}
\end{figure}

\subsubsection{\textbf{Custom Procedure}}

\begin{figure}[!h]
    \centering
    \includegraphics[width=\columnwidth]{figures/custom_procedure.pdf}
    \caption{ (left) \textbf{An Example of Custom Procedures} Here the \term{custom procedure} specifies the \term{base procedure} it builds upon, \term{decorators} for further customization, and \term{executions} that happen when the procedure passes or fails. Put them together, this \term{custom procedure} describes that three randomly selected juries from the channel will be asked to vote, and at least two affirmative votes from them are required for approval. If this procedure passes, it will summarize the vote results by posting a message in the channel subject to renaming. (middle) \textbf{An Example of Base Procedures} The \term{base procedure} \code{Jury} defines a list of \term{settings} that represent the required user input and a list of \term{variables} that describe its status. Note how a \term{setting} (in pink) is used and how a \term{variable} (in blue) is maintained in the procedure Code. (right up) \textbf{An Example of Decorators} It represents enforcing minimum procedure duration. Similar to decorators in Python, its code will be prepended to that of the \term{base procedure}. (right down) \textbf{An Example of Executions} It presents the \term{execution} \code{SlackPostMessage} that will happen when the procedure passes or fails.}
    \hfill
    \label{custom procedure}
\end{figure}

Figure \ref{custom procedure} shows an example of \term{custom procedures} in the form of declarative language. It specifies the \term{base procedure} this \term{custom procedure} builds upon, \code{Jury}, and the user configuration of its \term{settings}. The \term{base procedure} \code{Jury} also has the following JSON fields:  \code{name}, \code{description}, \term{settings}, and \term{variables}. As how a procedure is carried out depends on platforms, it has a \code{platform} field indicating platforms it can apply to.  

This \term{custom procedure} further customizes its \term{base procedure} \code{Jury} through two \term{decorators}--\code{Procedure duration} and \code{Voting notification}. We illustrate the JSON fields of the first \term{decorator} in the same figure.

Finally, this \term{custom procedure} sets \term{executions} when the procedure passes: posting a message summarizing the voting outcome.
